# Supplementary material for: Attention-based Fusion for Multi-source Human Image Generation
Source: arXiv:1905.02655 source file (2019-05-07)
Supplement: Supplementary file 1 [file fashionsupadditional.tex]

\begin{figure*}[h]
   \centering
   \setlength\tabcolsep{1.0pt}
   \resizebox{0.99\textwidth}{!}{\begin{tabular}{c|c|ccc|c}
     %% &&\multicolumn{4}{c|}{Market-1501}&\multicolumn{2}{c}{DeepFashion}\
     $x^i,i\in[1..3]$ & $x_\tau$ & $M_n=1$ & $M_n=2$ & $M_n=3$&  \small Attention Saliency\\ 

\includegraphics[height=0.24\columnwidth]{./figures/sup/comp/supp_3/input_fasionWOMENTeesTanksid0000300206_4full.png}&
\includegraphics[height=0.24\columnwidth]{./figures/sup/comp/supp_3/GT_fasionWOMENTeesTanksid0000300206_4full.png}&
\includegraphics[height=0.24\columnwidth]{./figures/sup/comp/supp_1/fasionWOMENTeesTanksid0000300206_4full.png}&
\includegraphics[height=0.24\columnwidth]{./figures/sup/comp/supp_2/fasionWOMENTeesTanksid0000300206_4full.png}&
\includegraphics[height=0.24\columnwidth]{./figures/sup/comp/supp_3/fasionWOMENTeesTanksid0000300206_4full.png}&
\includegraphics[height=0.24\columnwidth]{./figures/sup/comp/supp_3/att_fasionWOMENTeesTanksid0000300206_4full.png}
\\
%% \includegraphics[height=0.24\columnwidth]{./figures/sup/comp/supp_3/input_fasionWOMENDressesid0000409106_1front.png}&
%% \includegraphics[height=0.24\columnwidth]{./figures/sup/comp/supp_3/GT_fasionWOMENDressesid0000409106_1front.png}&
%% \includegraphics[height=0.24\columnwidth]{./figures/sup/comp/supp_1/fasionWOMENDressesid0000409106_1front.png}&
%% \includegraphics[height=0.24\columnwidth]{./figures/sup/comp/supp_2/fasionWOMENDressesid0000409106_1front.png}&
%% \includegraphics[height=0.24\columnwidth]{./figures/sup/comp/supp_3/fasionWOMENDressesid0000409106_1front.png}&
%% \includegraphics[height=0.24\columnwidth]{./figures/sup/comp/supp_3/att_fasionWOMENDressesid0000409106_1front.png}
%% \\
\includegraphics[height=0.24\columnwidth]{./figures/sup/comp/supp_3/input_fasionWOMENTeesTanksid0000660212_2side.png}&
\includegraphics[height=0.24\columnwidth]{./figures/sup/comp/supp_3/GT_fasionWOMENTeesTanksid0000660212_2side.png}&
\includegraphics[height=0.24\columnwidth]{./figures/sup/comp/supp_1/fasionWOMENTeesTanksid0000660212_2side.png}&
\includegraphics[height=0.24\columnwidth]{./figures/sup/comp/supp_2/fasionWOMENTeesTanksid0000660212_2side.png}&
\includegraphics[height=0.24\columnwidth]{./figures/sup/comp/supp_3/fasionWOMENTeesTanksid0000660212_2side.png}&
\includegraphics[height=0.24\columnwidth]{./figures/sup/comp/supp_3/att_fasionWOMENTeesTanksid0000660212_2side.png}
\\
\includegraphics[height=0.24\columnwidth]{./figures/sup/comp/supp_3/input_fasionWOMENSweatersid0000084004_2side.png}&
\includegraphics[height=0.24\columnwidth]{./figures/sup/comp/supp_3/GT_fasionWOMENSweatersid0000084004_2side.png}&
\includegraphics[height=0.24\columnwidth]{./figures/sup/comp/supp_1/fasionWOMENSweatersid0000084004_2side.png}&
\includegraphics[height=0.24\columnwidth]{./figures/sup/comp/supp_2/fasionWOMENSweatersid0000084004_2side.png}&
\includegraphics[height=0.24\columnwidth]{./figures/sup/comp/supp_3/fasionWOMENSweatersid0000084004_2side.png}&
\includegraphics[height=0.24\columnwidth]{./figures/sup/comp/supp_3/att_fasionWOMENSweatersid0000084004_2side.png}
\\
\includegraphics[height=0.24\columnwidth]{./figures/sup/comp/supp_3/input_fasionWOMENTeesTanksid0000512402_7additional.png}&
\includegraphics[height=0.24\columnwidth]{./figures/sup/comp/supp_3/GT_fasionWOMENTeesTanksid0000512402_7additional.png}&
\includegraphics[height=0.24\columnwidth]{./figures/sup/comp/supp_1/fasionWOMENTeesTanksid0000512402_7additional.png}&
\includegraphics[height=0.24\columnwidth]{./figures/sup/comp/supp_2/fasionWOMENTeesTanksid0000512402_7additional.png}&
\includegraphics[height=0.24\columnwidth]{./figures/sup/comp/supp_3/fasionWOMENTeesTanksid0000512402_7additional.png}&
\includegraphics[height=0.24\columnwidth]{./figures/sup/comp/supp_3/att_fasionWOMENTeesTanksid0000512402_7additional.png}
\\
\includegraphics[height=0.24\columnwidth]{./figures/sup/comp/supp_3/input_fasionWOMENDressesid0000689802_3back.png}&
\includegraphics[height=0.24\columnwidth]{./figures/sup/comp/supp_3/GT_fasionWOMENDressesid0000689802_3back.png}&
\includegraphics[height=0.24\columnwidth]{./figures/sup/comp/supp_1/fasionWOMENDressesid0000689802_3back.png}&
\includegraphics[height=0.24\columnwidth]{./figures/sup/comp/supp_2/fasionWOMENDressesid0000689802_3back.png}&
\includegraphics[height=0.24\columnwidth]{./figures/sup/comp/supp_3/fasionWOMENDressesid0000689802_3back.png}&
\includegraphics[height=0.24\columnwidth]{./figures/sup/comp/supp_3/att_fasionWOMENDressesid0000766701_4full.png}
\\
\includegraphics[height=0.24\columnwidth]{./figures/sup/comp/supp_3/input_fasionWOMENDressesid0000528102_1front.png}&
\includegraphics[height=0.24\columnwidth]{./figures/sup/comp/supp_3/GT_fasionWOMENDressesid0000528102_1front.png}&
\includegraphics[height=0.24\columnwidth]{./figures/sup/comp/supp_1/fasionWOMENDressesid0000528102_1front.png}&
\includegraphics[height=0.24\columnwidth]{./figures/sup/comp/supp_2/fasionWOMENDressesid0000528102_1front.png}&
\includegraphics[height=0.24\columnwidth]{./figures/sup/comp/supp_3/fasionWOMENDressesid0000528102_1front.png}&
\includegraphics[height=0.24\columnwidth]{./figures/sup/comp/supp_3/att_fasionWOMENDressesid0000528102_1front.png}
\\
\includegraphics[height=0.24\columnwidth]{./figures/sup/comp/supp_3/input_fasionWOMENBlousesShirtsid0000299703_3back.png}&
\includegraphics[height=0.24\columnwidth]{./figures/sup/comp/supp_3/GT_fasionWOMENBlousesShirtsid0000299703_3back.png}&
\includegraphics[height=0.24\columnwidth]{./figures/sup/comp/supp_1/fasionWOMENBlousesShirtsid0000299703_3back.png}&
\includegraphics[height=0.24\columnwidth]{./figures/sup/comp/supp_2/fasionWOMENBlousesShirtsid0000299703_3back.png}&
\includegraphics[height=0.24\columnwidth]{./figures/sup/comp/supp_3/fasionWOMENBlousesShirtsid0000299703_3back.png}&
\includegraphics[height=0.24\columnwidth]{./figures/sup/comp/supp_3/att_fasionWOMENBlousesShirtsid0000299703_3back.png}
\\

 \end{tabular}}
   \vspace{-0.4cm} 
   \caption{Additional qualitative results on the DeepFashion dataset.}
   \label{fig:fashionAdd}
  \end{figure*}
